# Supplementary material for: Search for a time-varying electron antineutrino signal at Daya Bay
Source: arXiv:1809.04660 ancillary file (2018-12-18)
Supplement: Supplementary file 1 [file SupplementalMaterial_SME.pdf]

# Daya Bay Reactor Neutrino Experiment

## Supplemental Material

August 2018

This document provides supplemental information for the article titled "Search for a time-varying electron antineutrino signal at Daya Bay". Section I provides the correlation matrices associated with the fit of the Standard-Model Extension presented in the article. All other sections provide information that is necessary to reproduce the fit.

**CONTENTS**

I. LV-CPTV COEFFICIENT CORRELATION MATRICES 2
II. RESIDUAL SURVIVAL PROBABILITY VS. SIDEREAL TIME 4
III. ANTINEUTRINO ENERGIES 6
IV. DIRECTIONAL FACTORS 6
V. PREDICTED REACTOR ANTINEUTRINO EVENT FRACTIONS 7
VI. BASELINES, TRANSITION AMPLITIUDES, AND EXPERIMENTAL FACTORS 9

# I. LV-CPTV COEFFICIENT CORRELATION MATRICES

This section provides the correlation matrices associated with the fits of the Standard-Model Extension described in Section IV and presented in Table II of the main text. Tables I through VI gives the matrices for each of the six flavor pairs.

TABLE I. Correlation matrix for the $\boldsymbol{ee}$ flavor pair.

| | | | | | | | | |
|---|---|---|---|---|---|---|---|---|
| $a_R^X$ | 1 | 0.77 | 0.16 | -0.01 | -0.02 | -0.05 | -0.00 | -0.00 |
| $c_R^{TX}$ | 0.77 | 1 | 0.73 | 0.01 | -0.00 | -0.12 | -0.00 | 0.00 |
| $c_R^{XZ}$ | 0.16 | 0.73 | 1 | 0.05 | 0.12 | 0.00 | 0.00 | 0.00 |
| $a_R^Y$ | -0.01 | 0.01 | 0.05 | 1 | 0.77 | 0.16 | 0.00 | 0.00 |
| $c_R^{TY}$ | -0.02 | -0.00 | 0.12 | 0.77 | 1 | 0.73 | 0.00 | 0.00 |
| $c_R^{YZ}$ | -0.05 | -0.12 | 0.00 | 0.16 | 0.73 | 1 | -0.00 | 0.00 |
| $c_R^{XX} - c_R^{YY}$ | -0.00 | -0.00 | 0.00 | 0.00 | 0.00 | -0.00 | 1 | -0.00 |
| $c_R^{XY}$ | -0.00 | 0.00 | 0.00 | 0.00 | 0.00 | 0.00 | -0.00 | 1 |

TABLE II. Correlation matrix for the $\boldsymbol{\mu\mu}$ flavor pair.

| | | | | | | | | |
|---|---|---|---|---|---|---|---|---|
| $a_R^X$ | 1 | 0.76 | 0.15 | -0.00 | -0.02 | -0.04 | -0.00 | 0.00 |
| $c_R^{TX}$ | 0.76 | 1 | 0.74 | 0.01 | -0.00 | -0.12 | -0.00 | 0.00 |
| $c_R^{XZ}$ | 0.15 | 0.74 | 1 | 0.04 | 0.12 | 0.00 | 0.00 | 0.00 |
| $a_R^Y$ | -0.00 | 0.01 | 0.04 | 1 | 0.76 | 0.15 | 0.00 | 0.00 |
| $c_R^{TY}$ | -0.02 | -0.00 | 0.12 | 0.76 | 1 | 0.73 | 0.00 | 0.00 |
| $c_R^{YZ}$ | -0.04 | -0.12 | 0.00 | 0.15 | 0.73 | 1 | -0.00 | 0.00 |
| $c_R^{XX} - c_R^{YY}$ | -0.00 | -0.00 | 0.00 | 0.00 | 0.00 | -0.00 | 1 | -0.00 |
| $c_R^{XY}$ | 0.00 | 0.00 | 0.00 | 0.00 | 0.00 | 0.00 | -0.00 | 1 |

TABLE III. Correlation matrix for the $\boldsymbol{\tau\tau}$ flavor pair.

| | | | | | | | | |
|---|---|---|---|---|---|---|---|---|
| $a_R^X$ | 1 | 0.78 | 0.18 | -0.00 | -0.02 | -0.05 | -0.00 | -0.00 |
| $c_R^{TX}$ | 0.78 | 1 | 0.73 | 0.02 | -0.00 | -0.12 | -0.00 | 0.00 |
| $c_R^{XZ}$ | 0.18 | 0.73 | 1 | 0.05 | 0.12 | 0.00 | 0.00 | 0.00 |
| $a_R^Y$ | -0.00 | 0.02 | 0.05 | 1 | 0.78 | 0.18 | 0.00 | 0.00 |
| $c_R^{TY}$ | -0.02 | -0.00 | 0.12 | 0.78 | 1 | 0.73 | 0.00 | 0.00 |
| $c_R^{YZ}$ | -0.05 | -0.12 | 0.00 | 0.18 | 0.73 | 1 | -0.00 | 0.00 |
| $c_R^{XX} - c_R^{YY}$ | -0.00 | -0.00 | 0.00 | 0.00 | 0.00 | -0.00 | 1 | -0.00 |
| $c_R^{XY}$ | -0.00 | 0.00 | 0.00 | 0.00 | 0.00 | 0.00 | -0.00 | 1 |

TABLE IV. Correlation matrix for the $\boldsymbol{e\mu}$ flavor pair.

| | | | | | | | | |
|---|---|---|---|---|---|---|---|---|
| $a_R^X$ | 1 | 0.88 | 0.10 | -0.00 | 0.02 | 0.04 | 0.00 | -0.00 |
| $c_R^{TX}$ | 0.88 | 1 | 0.50 | -0.03 | -0.00 | -0.05 | 0.00 | -0.00 |
| $c_R^{XZ}$ | 0.10 | 0.50 | 1 | -0.04 | 0.05 | -0.00 | 0.00 | 0.00 |
| $a_R^Y$ | -0.00 | -0.03 | -0.04 | 1 | 0.88 | 0.10 | -0.01 | 0.00 |
| $c_R^{TY}$ | 0.02 | -0.00 | 0.05 | 0.88 | 1 | 0.50 | -0.00 | 0.00 |
| $c_R^{YZ}$ | 0.04 | -0.05 | -0.00 | 0.10 | 0.50 | 1 | -0.00 | 0.00 |
| $c_R^{XX} - c_R^{YY}$ | 0.00 | 0.00 | 0.00 | -0.01 | -0.00 | -0.00 | 1 | -0.00 |
| $c_R^{XY}$ | -0.00 | -0.00 | 0.00 | 0.00 | 0.00 | 0.00 | -0.00 | 1 |

TABLE V. Correlation matrix for the $\boldsymbol{e\tau}$ flavor pair.

| | | | | | | | | |
|---|---|---|---|---|---|---|---|---|
| $a_R^X$ | 1 | 0.90 | 0.14 | -0.00 | 0.03 | 0.05 | 0.00 | -0.00 |
| $c_R^{TX}$ | 0.90 | 1 | 0.49 | -0.03 | -0.00 | -0.03 | 0.00 | -0.00 |
| $c_R^{XZ}$ | 0.14 | 0.49 | 1 | -0.05 | 0.03 | -0.00 | 0.00 | 0.00 |
| $a_R^Y$ | -0.00 | -0.03 | -0.05 | 1 | 0.90 | 0.14 | -0.01 | 0.00 |
| $c_R^{TY}$ | 0.03 | -0.00 | 0.03 | 0.90 | 1 | 0.49 | -0.01 | 0.00 |
| $c_R^{YZ}$ | 0.05 | -0.03 | -0.00 | 0.14 | 0.49 | 1 | -0.00 | -0.00 |
| $c_R^{XX} - c_R^{YY}$ | 0.00 | 0.00 | 0.00 | -0.01 | -0.01 | -0.00 | 1 | -0.00 |
| $c_R^{XY}$ | -0.00 | -0.00 | 0.00 | 0.00 | 0.00 | -0.00 | -0.00 | 1 |

TABLE VI. Correlation matrix for the $\boldsymbol{\mu\tau}$ flavor pair.

| | | | | | | | | |
|---|---|---|---|---|---|---|---|---|
| $a_R^X$ | 1 | 0.77 | 0.16 | -0.00 | -0.02 | -0.05 | -0.00 | 0.00 |
| $c_R^{TX}$ | 0.77 | 1 | 0.73 | 0.01 | -0.00 | -0.12 | -0.00 | 0.00 |
| $c_R^{XZ}$ | 0.16 | 0.73 | 1 | 0.05 | 0.12 | 0.00 | 0.00 | 0.00 |
| $a_R^Y$ | -0.00 | 0.01 | 0.05 | 1 | 0.77 | 0.16 | 0.00 | 0.00 |
| $c_R^{TY}$ | -0.02 | -0.00 | 0.12 | 0.77 | 1 | 0.73 | 0.00 | 0.00 |
| $c_R^{YZ}$ | -0.05 | -0.12 | 0.00 | 0.16 | 0.73 | 1 | -0.00 | 0.00 |
| $c_R^{XX} - c_R^{YY}$ | -0.00 | -0.00 | 0.00 | 0.00 | 0.00 | -0.00 | 1 | -0.00 |
| $c_R^{XY}$ | 0.00 | 0.00 | 0.00 | 0.00 | 0.00 | 0.00 | -0.00 | 1 |

## II. RESIDUAL SURVIVAL PROBABILITY VS. SIDEREAL TIME

Tables VII, VIII, and IX provide the residual survival probability of reactor $\overline{\nu}_e$, $R$, in 24 sidereal hour bins and 5 energy bins, for each experimental hall. These are the same $R$ shown in Fig. 5 and used in Eq. (5) of the main text. The energy bins are defined in Table X. The errors include both statistical and systematic components.

TABLE VII. Residual survival probability of $\overline{\nu}_e$ in **experimental hall 1** vs. sidereal hour and energy bin.

| Time bin | $E$ bin 1 | $E$ bin 2 | $E$ bin 3 | $E$ bin 4 | $E$ bin 5 |
|---|---|---|---|---|---|
| 1 | -0.0033 ± 0.0160 | -0.0060 ± 0.0122 | -0.0010 ± 0.0123 | 0.0033 ± 0.0147 | -0.0058 ± 0.0166 |
| 2 | -0.0027 ± 0.0161 | -0.0003 ± 0.0122 | 0.0049 ± 0.0122 | 0.0124 ± 0.0146 | 0.0133 ± 0.0165 |
| 3 | 0.0085 ± 0.0160 | -0.0027 ± 0.0122 | 0.0077 ± 0.0122 | -0.0176 ± 0.0149 | 0.0016 ± 0.0166 |
| 4 | -0.0138 ± 0.0162 | 0.0237 ± 0.0121 | -0.0118 ± 0.0124 | -0.0174 ± 0.0149 | 0.0003 ± 0.0166 |
| 5 | -0.0082 ± 0.0162 | 0.0110 ± 0.0122 | -0.0024 ± 0.0123 | -0.0097 ± 0.0149 | 0.0278 ± 0.0164 |
| 6 | -0.0084 ± 0.0162 | 0.0092 ± 0.0122 | 0.0051 ± 0.0123 | 0.0124 ± 0.0148 | 0.0170 ± 0.0166 |
| 7 | -0.0000 ± 0.0162 | 0.0002 ± 0.0123 | -0.0109 ± 0.0125 | -0.0131 ± 0.0150 | -0.0068 ± 0.0168 |
| 8 | 0.0145 ± 0.0162 | 0.0062 ± 0.0123 | -0.0069 ± 0.0125 | -0.0006 ± 0.0150 | 0.0252 ± 0.0166 |
| 9 | 0.0212 ± 0.0161 | 0.0150 ± 0.0123 | 0.0074 ± 0.0124 | 0.0226 ± 0.0148 | 0.0122 ± 0.0167 |
| 10 | 0.0029 ± 0.0163 | 0.0011 ± 0.0124 | 0.0015 ± 0.0125 | -0.0005 ± 0.0150 | -0.0055 ± 0.0169 |
| 11 | -0.0028 ± 0.0163 | -0.0017 ± 0.0123 | 0.0043 ± 0.0124 | -0.0221 ± 0.0151 | 0.0103 ± 0.0167 |
| 12 | 0.0041 ± 0.0161 | -0.0244 ± 0.0124 | 0.0055 ± 0.0123 | -0.0072 ± 0.0149 | 0.0044 ± 0.0167 |
| 13 | 0.0162 ± 0.0160 | 0.0035 ± 0.0122 | -0.0099 ± 0.0124 | 0.0004 ± 0.0148 | -0.0115 ± 0.0168 |
| 14 | -0.0099 ± 0.0162 | 0.0043 ± 0.0122 | -0.0128 ± 0.0124 | 0.0177 ± 0.0147 | -0.0326 ± 0.0170 |
| 15 | 0.0136 ± 0.0160 | 0.0001 ± 0.0122 | 0.0039 ± 0.0123 | 0.0145 ± 0.0147 | 0.0182 ± 0.0165 |
| 16 | 0.0097 ± 0.0160 | 0.0038 ± 0.0122 | 0.0117 ± 0.0122 | -0.0031 ± 0.0148 | 0.0120 ± 0.0165 |
| 17 | 0.0114 ± 0.0160 | -0.0132 ± 0.0123 | 0.0064 ± 0.0123 | -0.0373 ± 0.0151 | -0.0046 ± 0.0167 |
| 18 | -0.0241 ± 0.0163 | -0.0002 ± 0.0122 | -0.0029 ± 0.0123 | 0.0134 ± 0.0147 | -0.0258 ± 0.0168 |
| 19 | -0.0266 ± 0.0163 | 0.0084 ± 0.0122 | -0.0038 ± 0.0123 | 0.0155 ± 0.0147 | -0.0126 ± 0.0167 |
| 20 | 0.0079 ± 0.0160 | -0.0001 ± 0.0122 | 0.0041 ± 0.0123 | -0.0004 ± 0.0147 | -0.0287 ± 0.0168 |
| 21 | -0.0010 ± 0.0160 | -0.0117 ± 0.0123 | -0.0075 ± 0.0123 | -0.0051 ± 0.0148 | -0.0088 ± 0.0167 |
| 22 | -0.0082 ± 0.0161 | -0.0142 ± 0.0123 | 0.0013 ± 0.0123 | 0.0002 ± 0.0147 | -0.0151 ± 0.0167 |
| 23 | -0.0157 ± 0.0162 | -0.0113 ± 0.0122 | 0.0111 ± 0.0122 | -0.0029 ± 0.0147 | 0.0074 ± 0.0165 |
| 24 | 0.0215 ± 0.0158 | 0.0030 ± 0.0121 | -0.0016 ± 0.0122 | 0.0292 ± 0.0145 | 0.0180 ± 0.0164 |

TABLE VIII. Residual survival probability of $\overline{\nu}_e$ in **experimental hall 2** vs. sidereal hour and energy bin.

| Time bin | $E$ bin 1 | $E$ bin 2 | $E$ bin 3 | $E$ bin 4 | $E$ bin 5 |
|---|---|---|---|---|---|
| 1 | -0.0004 ± 0.0182 | -0.0170 ± 0.0139 | 0.0054 ± 0.0139 | 0.0171 ± 0.0167 | -0.0178 ± 0.0189 |
| 2 | 0.0225 ± 0.0180 | 0.0013 ± 0.0137 | 0.0000 ± 0.0139 | 0.0074 ± 0.0167 | -0.0308 ± 0.0190 |
| 3 | -0.0061 ± 0.0182 | -0.0168 ± 0.0138 | 0.0103 ± 0.0138 | 0.0027 ± 0.0167 | -0.0089 ± 0.0188 |
| 4 | 0.0097 ± 0.0181 | -0.0012 ± 0.0137 | -0.0081 ± 0.0139 | -0.0058 ± 0.0168 | 0.0133 ± 0.0186 |
| 5 | -0.0255 ± 0.0185 | -0.0140 ± 0.0139 | -0.0050 ± 0.0139 | -0.0083 ± 0.0169 | 0.0119 ± 0.0186 |
| 6 | -0.0028 ± 0.0182 | -0.0047 ± 0.0138 | 0.0221 ± 0.0137 | -0.0349 ± 0.0171 | 0.0152 ± 0.0186 |
| 7 | -0.0106 ± 0.0184 | -0.0093 ± 0.0139 | -0.0160 ± 0.0140 | 0.0078 ± 0.0168 | 0.0231 ± 0.0186 |
| 8 | -0.0320 ± 0.0186 | -0.0011 ± 0.0138 | -0.0114 ± 0.0140 | 0.0140 ± 0.0167 | 0.0207 ± 0.0186 |
| 9 | -0.0169 ± 0.0184 | -0.0152 ± 0.0139 | -0.0174 ± 0.0140 | 0.0162 ± 0.0167 | 0.0085 ± 0.0187 |
| 10 | -0.0264 ± 0.0185 | 0.0173 ± 0.0137 | -0.0045 ± 0.0139 | -0.0013 ± 0.0168 | -0.0149 ± 0.0189 |
| 11 | 0.0234 ± 0.0180 | -0.0099 ± 0.0138 | 0.0141 ± 0.0138 | -0.0121 ± 0.0169 | 0.0264 ± 0.0185 |
| 12 | 0.0165 ± 0.0180 | -0.0087 ± 0.0138 | 0.0098 ± 0.0138 | 0.0153 ± 0.0166 | 0.0279 ± 0.0184 |
| 13 | 0.0222 ± 0.0179 | 0.0100 ± 0.0136 | 0.0144 ± 0.0137 | -0.0227 ± 0.0169 | -0.0014 ± 0.0186 |
| 14 | -0.0151 ± 0.0183 | 0.0102 ± 0.0136 | -0.0052 ± 0.0139 | 0.0142 ± 0.0166 | -0.0093 ± 0.0188 |
| 15 | -0.0348 ± 0.0185 | 0.0227 ± 0.0136 | -0.0101 ± 0.0139 | 0.0123 ± 0.0166 | -0.0475 ± 0.0191 |
| 16 | 0.0318 ± 0.0179 | -0.0071 ± 0.0138 | -0.0119 ± 0.0139 | 0.0057 ± 0.0167 | -0.0167 ± 0.0188 |
| 17 | 0.0052 ± 0.0182 | 0.0196 ± 0.0136 | 0.0146 ± 0.0138 | -0.0215 ± 0.0170 | 0.0291 ± 0.0185 |
| 18 | -0.0010 ± 0.0182 | -0.0011 ± 0.0138 | -0.0209 ± 0.0140 | -0.0166 ± 0.0169 | 0.0217 ± 0.0185 |
| 19 | -0.0121 ± 0.0184 | 0.0033 ± 0.0137 | -0.0023 ± 0.0139 | 0.0118 ± 0.0167 | -0.0063 ± 0.0188 |
| 20 | -0.0029 ± 0.0182 | -0.0045 ± 0.0138 | 0.0043 ± 0.0138 | 0.0092 ± 0.0167 | 0.0094 ± 0.0186 |
| 21 | 0.0404 ± 0.0178 | 0.0153 ± 0.0136 | 0.0203 ± 0.0137 | -0.0117 ± 0.0168 | -0.0041 ± 0.0187 |
| 22 | 0.0019 ± 0.0181 | 0.0366 ± 0.0134 | 0.0174 ± 0.0137 | -0.0046 ± 0.0167 | -0.0242 ± 0.0189 |
| 23 | 0.0147 ± 0.0180 | -0.0042 ± 0.0137 | -0.0171 ± 0.0139 | 0.0022 ± 0.0167 | -0.0378 ± 0.0190 |
| 24 | 0.0035 ± 0.0182 | -0.0180 ± 0.0139 | 0.0013 ± 0.0139 | 0.0104 ± 0.0167 | 0.0198 ± 0.0185 |

TABLE IX. Residual survival probability of $\overline{\nu}_e$ in **experimental hall 3** vs. sidereal hour and energy bin.

| Time bin | $E$ bin 1 | $E$ bin 2 | $E$ bin 3 | $E$ bin 4 | $E$ bin 5 |
|---|---|---|---|---|---|
| 1 | -0.0342 ± 0.0333 | 0.0037 ± 0.0233 | 0.0278 ± 0.0230 | -0.0254 ± 0.0287 | -0.0449 ± 0.0325 |
| 2 | -0.0181 ± 0.0329 | 0.0040 ± 0.0233 | 0.0268 ± 0.0229 | 0.0450 ± 0.0276 | 0.0007 ± 0.0317 |
| 3 | 0.0085 ± 0.0323 | -0.0252 ± 0.0235 | 0.0586 ± 0.0225 | -0.0202 ± 0.0285 | 0.0021 ± 0.0316 |
| 4 | 0.0174 ± 0.0322 | 0.0405 ± 0.0227 | -0.0369 ± 0.0237 | 0.0022 ± 0.0282 | -0.0263 ± 0.0321 |
| 5 | -0.0439 ± 0.0334 | -0.0271 ± 0.0237 | -0.0140 ± 0.0235 | 0.0182 ± 0.0281 | 0.0696 ± 0.0306 |
| 6 | -0.0007 ± 0.0327 | -0.0044 ± 0.0234 | -0.0149 ± 0.0235 | 0.0320 ± 0.0279 | -0.0267 ± 0.0322 |
| 7 | 0.0275 ± 0.0322 | -0.0304 ± 0.0238 | -0.0085 ± 0.0235 | 0.0027 ± 0.0283 | -0.0050 ± 0.0319 |
| 8 | -0.0036 ± 0.0329 | 0.0187 ± 0.0233 | -0.0176 ± 0.0238 | 0.0136 ± 0.0283 | 0.0203 ± 0.0317 |
| 9 | 0.0113 ± 0.0325 | -0.0066 ± 0.0235 | -0.0008 ± 0.0234 | 0.0180 ± 0.0282 | 0.0024 ± 0.0319 |
| 10 | 0.0252 ± 0.0323 | 0.0409 ± 0.0229 | 0.0236 ± 0.0231 | -0.0293 ± 0.0289 | 0.0218 ± 0.0315 |
| 11 | 0.0098 ± 0.0326 | 0.0029 ± 0.0233 | -0.0093 ± 0.0235 | 0.0377 ± 0.0278 | 0.0042 ± 0.0317 |
| 12 | -0.0250 ± 0.0331 | -0.0033 ± 0.0234 | 0.0225 ± 0.0231 | 0.0227 ± 0.0280 | -0.0014 ± 0.0318 |
| 13 | -0.0036 ± 0.0325 | -0.0121 ± 0.0234 | -0.0195 ± 0.0235 | 0.0027 ± 0.0282 | -0.0175 ± 0.0319 |
| 14 | 0.0305 ± 0.0320 | -0.0272 ± 0.0237 | -0.0099 ± 0.0234 | -0.0522 ± 0.0291 | 0.0715 ± 0.0305 |
| 15 | -0.0511 ± 0.0335 | -0.0172 ± 0.0235 | -0.0486 ± 0.0239 | -0.0517 ± 0.0291 | 0.0490 ± 0.0308 |
| 16 | 0.0500 ± 0.0316 | -0.0047 ± 0.0233 | 0.0097 ± 0.0231 | -0.0026 ± 0.0283 | 0.0117 ± 0.0314 |
| 17 | -0.0266 ± 0.0332 | 0.0408 ± 0.0228 | -0.0264 ± 0.0236 | 0.0060 ± 0.0282 | 0.0128 ± 0.0315 |
| 18 | -0.0204 ± 0.0330 | 0.0189 ± 0.0232 | 0.0216 ± 0.0231 | -0.0147 ± 0.0286 | -0.0483 ± 0.0327 |
| 19 | 0.0567 ± 0.0318 | -0.0100 ± 0.0235 | 0.0166 ± 0.0232 | 0.0154 ± 0.0282 | -0.0150 ± 0.0321 |
| 20 | 0.0125 ± 0.0323 | -0.0119 ± 0.0234 | 0.0158 ± 0.0230 | 0.0383 ± 0.0277 | -0.0147 ± 0.0318 |
| 21 | 0.0031 ± 0.0325 | 0.0452 ± 0.0227 | 0.0380 ± 0.0228 | 0.0038 ± 0.0283 | -0.0139 ± 0.0320 |
| 22 | 0.0136 ± 0.0322 | -0.0228 ± 0.0235 | -0.0363 ± 0.0236 | -0.0295 ± 0.0286 | -0.0069 ± 0.0316 |
| 23 | -0.0094 ± 0.0326 | 0.0331 ± 0.0228 | -0.0024 ± 0.0232 | -0.0043 ± 0.0283 | 0.0076 ± 0.0315 |
| 24 | 0.0561 ± 0.0317 | 0.0001 ± 0.0233 | 0.0262 ± 0.0229 | 0.0249 ± 0.0279 | 0.0093 ± 0.0316 |

## III. ANTINEUTRINO ENERGIES

Table X lists the mean $\overline{\nu}_e$ energy corresponding to the selected prompt energy bins introduced in Section IV and illustrated in Fig. 5 of the main text. The root mean square (RMS) of each mean $\overline{\nu}_e$ energy is also listed.

TABLE X. Prompt energy bins and corresponding mean $\overline{\nu}_e$ energies.

| $E$ Bin | $E_{\text{prompt}}$[MeV] | $E_{\bar{\nu}_e}$[MeV] | $\text{RMS}_{\bar{E}_{\bar{\nu}_e}}$[MeV] |
|---|---|---|---|
| 1 | (0.7, 2.0) | 2.55 | 0.53 |
| 2 | (2.0, 3.0) | 3.36 | 0.37 |
| 3 | (3.0, 4.0) | 4.30 | 0.35 |
| 4 | (4.0, 5.0) | 5.28 | 0.35 |
| 5 | (5.0, 12.0) | 6.57 | 0.63 |

## IV. DIRECTIONAL FACTORS

Table XI lists the directional factors for each reactor-hall pair. They were calculated following Eq. (A9) of the main text.

TABLE XI. Directional factors for each reactor-hall pair.

| Hall | Reactor | $\hat{N}^X$ | $\hat{N}^Y$ | $\hat{N}^Z$ |
|---|---|---|---|---|
| EH1 | D1 | -0.461 | -0.004 | 0.887 |
| EH1 | D2 | -0.448 | 0.236 | 0.862 |
| EH1 | L1 | 0.221 | -0.753 | -0.620 |
| EH1 | L2 | 0.210 | -0.769 | -0.604 |
| EH1 | L3 | 0.265 | -0.668 | -0.696 |
| EH1 | L4 | 0.261 | -0.673 | -0.692 |
| EH2 | D1 | -0.390 | 0.263 | 0.883 |
| EH2 | D2 | -0.382 | 0.323 | 0.866 |
| EH2 | L1 | -0.329 | -0.698 | 0.636 |
| EH2 | L2 | -0.370 | -0.560 | 0.741 |
| EH2 | L3 | 0.008 | -0.989 | -0.149 |
| EH2 | L4 | -0.046 | -0.998 | -0.034 |
| EH3 | D1 | -0.379 | -0.303 | 0.874 |
| EH3 | D2 | -0.384 | -0.260 | 0.886 |
| EH3 | L1 | -0.236 | -0.820 | 0.521 |
| EH3 | L2 | -0.254 | -0.786 | 0.564 |
| EH3 | L3 | -0.131 | -0.954 | 0.269 |
| EH3 | L4 | -0.151 | -0.936 | 0.317 |

## V. PREDICTED REACTOR ANTINEUTRINO EVENT FRACTIONS

Tables XII, XIII, and XIV provide the predicted fractions of inverse beta decays, $f$, in each experimental hall (EH) and each sidereal time bin, originating from each nuclear reactor as defined by Eq. (4) in Section IV of the main text. See Fig. 1 of the main text for the relative location of each reactor.

TABLE XII. Predicted fractions of inverse beta decays in **experimental hall 1** and time bin, originating from each nuclear reactor.

| Time bin | D1 | D2 | L1 | L2 | L3 | L4 |
|---|---|---|---|---|---|---|
| 1 | 0.389 | 0.405 | 0.063 | 0.082 | 0.030 | 0.031 |
| 2 | 0.389 | 0.405 | 0.063 | 0.082 | 0.030 | 0.031 |
| 3 | 0.387 | 0.406 | 0.063 | 0.083 | 0.030 | 0.031 |
| 4 | 0.387 | 0.406 | 0.063 | 0.083 | 0.030 | 0.031 |
| 5 | 0.387 | 0.406 | 0.063 | 0.083 | 0.030 | 0.031 |
| 6 | 0.386 | 0.406 | 0.064 | 0.083 | 0.030 | 0.031 |
| 7 | 0.386 | 0.406 | 0.064 | 0.083 | 0.030 | 0.031 |
| 8 | 0.386 | 0.406 | 0.064 | 0.083 | 0.030 | 0.030 |
| 9 | 0.385 | 0.407 | 0.064 | 0.083 | 0.030 | 0.031 |
| 10 | 0.384 | 0.408 | 0.064 | 0.083 | 0.030 | 0.031 |
| 11 | 0.385 | 0.408 | 0.063 | 0.082 | 0.030 | 0.031 |
| 12 | 0.386 | 0.408 | 0.063 | 0.082 | 0.030 | 0.031 |
| 13 | 0.387 | 0.408 | 0.063 | 0.082 | 0.030 | 0.031 |
| 14 | 0.388 | 0.407 | 0.062 | 0.081 | 0.030 | 0.031 |
| 15 | 0.389 | 0.406 | 0.062 | 0.081 | 0.030 | 0.031 |
| 16 | 0.389 | 0.406 | 0.062 | 0.082 | 0.030 | 0.031 |
| 17 | 0.389 | 0.406 | 0.062 | 0.082 | 0.030 | 0.031 |
| 18 | 0.388 | 0.407 | 0.062 | 0.082 | 0.030 | 0.031 |
| 19 | 0.388 | 0.407 | 0.062 | 0.082 | 0.030 | 0.031 |
| 20 | 0.387 | 0.407 | 0.063 | 0.082 | 0.030 | 0.031 |
| 21 | 0.387 | 0.406 | 0.063 | 0.082 | 0.030 | 0.031 |
| 22 | 0.387 | 0.407 | 0.063 | 0.082 | 0.030 | 0.031 |
| 23 | 0.387 | 0.407 | 0.063 | 0.082 | 0.030 | 0.031 |
| 24 | 0.388 | 0.407 | 0.063 | 0.082 | 0.030 | 0.031 |

TABLE XIII. Predicted fractions of inverse beta decays in **experimental hall 2** and time bin, originating from each nuclear reactor.

| Time bin | D1 | D2 | L1 | L2 | L3 | L4 |
|---|---|---|---|---|---|---|
| 1 | 0.033 | 0.033 | 0.257 | 0.254 | 0.197 | 0.227 |
| 2 | 0.033 | 0.033 | 0.258 | 0.254 | 0.196 | 0.227 |
| 3 | 0.033 | 0.033 | 0.258 | 0.254 | 0.196 | 0.226 |
| 4 | 0.032 | 0.033 | 0.257 | 0.257 | 0.196 | 0.226 |
| 5 | 0.032 | 0.033 | 0.257 | 0.256 | 0.196 | 0.226 |
| 6 | 0.032 | 0.033 | 0.259 | 0.255 | 0.196 | 0.226 |
| 7 | 0.032 | 0.033 | 0.260 | 0.255 | 0.195 | 0.225 |
| 8 | 0.032 | 0.033 | 0.261 | 0.254 | 0.196 | 0.224 |
| 9 | 0.032 | 0.033 | 0.261 | 0.254 | 0.196 | 0.225 |
| 10 | 0.032 | 0.033 | 0.260 | 0.254 | 0.195 | 0.227 |
| 11 | 0.032 | 0.033 | 0.259 | 0.253 | 0.195 | 0.228 |
| 12 | 0.032 | 0.033 | 0.259 | 0.253 | 0.196 | 0.227 |
| 13 | 0.032 | 0.033 | 0.258 | 0.253 | 0.196 | 0.227 |
| 14 | 0.033 | 0.033 | 0.257 | 0.253 | 0.197 | 0.228 |
| 15 | 0.032 | 0.033 | 0.256 | 0.253 | 0.197 | 0.228 |
| 16 | 0.032 | 0.033 | 0.256 | 0.254 | 0.196 | 0.228 |
| 17 | 0.033 | 0.033 | 0.256 | 0.254 | 0.196 | 0.228 |
| 18 | 0.032 | 0.033 | 0.256 | 0.254 | 0.196 | 0.228 |
| 19 | 0.032 | 0.033 | 0.256 | 0.254 | 0.196 | 0.229 |
| 20 | 0.032 | 0.033 | 0.256 | 0.254 | 0.196 | 0.229 |
| 21 | 0.032 | 0.033 | 0.256 | 0.253 | 0.196 | 0.229 |
| 22 | 0.032 | 0.033 | 0.257 | 0.253 | 0.196 | 0.229 |
| 23 | 0.032 | 0.033 | 0.257 | 0.253 | 0.196 | 0.228 |
| 24 | 0.033 | 0.033 | 0.257 | 0.254 | 0.196 | 0.228 |

TABLE XIV. Predicted fractions of inverse beta decays in **experimental hall 3** and time bin, originating from each nuclear reactor.

| Time bin | D1 | D2 | L1 | L2 | L3 | L4 |
|---|---|---|---|---|---|---|
| 1 | 0.118 | 0.130 | 0.183 | 0.197 | 0.193 | 0.180 |
| 2 | 0.118 | 0.129 | 0.183 | 0.197 | 0.193 | 0.180 |
| 3 | 0.117 | 0.129 | 0.184 | 0.197 | 0.193 | 0.180 |
| 4 | 0.116 | 0.129 | 0.183 | 0.199 | 0.193 | 0.179 |
| 5 | 0.117 | 0.129 | 0.183 | 0.199 | 0.193 | 0.180 |
| 6 | 0.116 | 0.129 | 0.185 | 0.198 | 0.193 | 0.179 |
| 7 | 0.116 | 0.129 | 0.186 | 0.198 | 0.193 | 0.179 |
| 8 | 0.116 | 0.129 | 0.187 | 0.197 | 0.193 | 0.178 |
| 9 | 0.115 | 0.129 | 0.187 | 0.197 | 0.193 | 0.179 |
| 10 | 0.115 | 0.129 | 0.186 | 0.197 | 0.192 | 0.181 |
| 11 | 0.115 | 0.130 | 0.185 | 0.196 | 0.192 | 0.181 |
| 12 | 0.116 | 0.130 | 0.184 | 0.197 | 0.192 | 0.181 |
| 13 | 0.117 | 0.130 | 0.184 | 0.196 | 0.193 | 0.181 |
| 14 | 0.117 | 0.131 | 0.183 | 0.195 | 0.193 | 0.181 |
| 15 | 0.117 | 0.130 | 0.182 | 0.196 | 0.193 | 0.182 |
| 16 | 0.117 | 0.130 | 0.182 | 0.196 | 0.193 | 0.182 |
| 17 | 0.117 | 0.130 | 0.182 | 0.196 | 0.193 | 0.182 |
| 18 | 0.117 | 0.130 | 0.182 | 0.196 | 0.193 | 0.182 |
| 19 | 0.117 | 0.130 | 0.182 | 0.196 | 0.192 | 0.182 |
| 20 | 0.117 | 0.130 | 0.183 | 0.196 | 0.192 | 0.182 |
| 21 | 0.117 | 0.130 | 0.182 | 0.197 | 0.193 | 0.182 |
| 22 | 0.116 | 0.130 | 0.182 | 0.197 | 0.193 | 0.182 |
| 23 | 0.117 | 0.130 | 0.182 | 0.197 | 0.193 | 0.182 |
| 24 | 0.117 | 0.130 | 0.182 | 0.197 | 0.193 | 0.181 |

## VI. BASELINES, TRANSITION AMPLITIUDES, AND EXPERIMENTAL FACTORS

Table XV lists the baselines $L$, and transition amplitudes $S_{ee}^{(0)}$ with experimental factors $\mathcal{M}_{ee}^{(1)}$, for each flavor pair and each reactor-hall pair (see Fig. 1 of the main text for the layout). The calculation of the latter two quantites followed Eqs. (A3) and (A5) of the main text. Neutrino oscillation parameters are from PDG 2015 ($\sin^2 2\theta_{12} = 0.846 \pm 0.021, \sin^2 2\theta_{23} = 0.999^{+0.001}_{-0.018}, \sin^2 2\theta_{13} = 0.085 \pm 0.005, \Delta m^2_{21} = (7.53 \pm 0.18) \times 10^{-5}\text{eV}^2, \Delta m^2_{32} = (2.42 \pm 0.06) \times 10^{-3}\text{eV}^2$) assuming normal neutrino mass ordering. We took the CP violating phase to be zero. The average antineutrino energy is 4.2 MeV.

TABLE XV. The baselines, transition amplitudes, and experimental factors for each flavor pair and each reactor-hall pair.

| Hall | Reactor | $L$[m] | $\lvert S_{ee}^{(0)}\rvert^2$ | $\text{Im}(S_{ee}^{(0)*}(\mathcal{M}_{ee}^{(1)})_{cd})$ | | | | | |
|---|---|---|---|---|---|---|---|---|---|
| | | | | $ee$ | $\mu\mu$ | $\tau\tau$ | $e\mu$ | $e\tau$ | $\mu\tau$ |
| EH1 | D1 | 360.2 | 0.994 | 0.0146 | -0.0054 | -0.0092 | 0.0182 | 0.0279 | -0.0138 |
| EH1 | D2 | 370.1 | 0.994 | 0.0150 | -0.0055 | -0.0095 | 0.0187 | 0.0286 | -0.0141 |
| EH1 | L1 | 903.4 | 0.967 | 0.0325 | -0.0122 | -0.0203 | 0.0408 | 0.0614 | -0.0271 |
| EH1 | L2 | 817.0 | 0.972 | 0.0302 | -0.0113 | -0.0189 | 0.0378 | 0.0571 | -0.0259 |
| EH1 | L3 | 1353.9 | 0.938 | 0.0407 | -0.0157 | -0.0250 | 0.0513 | 0.0756 | -0.0268 |
| EH1 | L4 | 1265.6 | 0.944 | 0.0397 | -0.0152 | -0.0244 | 0.0499 | 0.0739 | -0.0278 |
| EH2 | D1 | 1335.0 | 0.940 | 0.0405 | -0.0156 | -0.0249 | 0.0510 | 0.0753 | -0.0271 |
| EH2 | D2 | 1360.5 | 0.938 | 0.0408 | -0.0158 | -0.0250 | 0.0513 | 0.0757 | -0.0267 |
| EH2 | L1 | 470.3 | 0.990 | 0.0188 | -0.0069 | -0.0118 | 0.0234 | 0.0358 | -0.0175 |
| EH2 | L2 | 492.5 | 0.989 | 0.0196 | -0.0073 | -0.0123 | 0.0245 | 0.0373 | -0.0182 |
| EH2 | L3 | 558.1 | 0.986 | 0.0219 | -0.0081 | -0.0138 | 0.0274 | 0.0417 | -0.0201 |
| EH2 | L4 | 500.1 | 0.989 | 0.0199 | -0.0074 | -0.0125 | 0.0248 | 0.0378 | -0.0184 |
| EH3 | D1 | 1921.4 | 0.915 | 0.0418 | -0.0170 | -0.0249 | 0.0509 | 0.0737 | -0.0123 |
| EH3 | D2 | 1895.9 | 0.916 | 0.0420 | -0.0170 | -0.0250 | 0.0513 | 0.0742 | -0.0132 |
| EH3 | L1 | 1536.9 | 0.929 | 0.0422 | -0.0165 | -0.0256 | 0.0528 | 0.0773 | -0.0236 |
| EH3 | L2 | 1537.2 | 0.929 | 0.0422 | -0.0165 | -0.0256 | 0.0528 | 0.0773 | -0.0236 |
| EH3 | L3 | 1555.6 | 0.928 | 0.0422 | -0.0166 | -0.0257 | 0.0529 | 0.0773 | -0.0232 |
| EH3 | L4 | 1529.1 | 0.929 | 0.0421 | -0.0165 | -0.0256 | 0.0528 | 0.0773 | -0.0238 |
